# Supplementary material for: Distortion and destruction of colloidal flocks in disordered environments
Source: arXiv:1610.04404 ancillary file (2016-10-14)
Supplement: Supplementary file 1 [file Supplementary_Information.pdf]

# Supplementary Informations


**1 Supplementary Methods** **2**

**2 Supplementary Note 1: Flocking-through-disorder experiments** **2**

2.1 Global flock morphology: current, density and polarization fields . . . 2

2.2 Isotropy of the current field above $\phi_o^\star$ . . . 4

2.3 Obstacle-Roller Scattering and Effective Diffusion . . . 5

**3 Supplementary Note 2: Flocking-through-disorder theory** **6**

3.1 Equations of motion of interacting colloidal rollers in a homogeneous media . . . 6

3.2 Roller-obstacle interactions . . . 6

3.3 Flocking transition in weak quenched disorder . . . 7

3.3.1 Kinetic theory . . . 7

3.3.2 Hydrodynamic theory . . . 8

3.3.3 Flock morphologies . . . 8

3.4 Emergence of flowing-channel networks . . . 10

3.4.1 Hydrodynamics of a strongly polarized flock of rollers: homogeneous media . . . 10

3.4.2 Hydrodynamics of a strongly polarized flock of rollers: heterogeneous media . . . 10

3.4.3 Response to a quenched random field and formation of sparse river networks . . . 11

3.5 Disorder-induced melting and emergent river networks: a robust picture . . . 12

**4 Supplementary Note 3: Flocking through periodic lattices** **12**

**5 Description of the supplementary videos** **14**

**Supplementary References** **14**

# 1 Supplementary Methods

We sketch the microfluidic device used to handle the colloidal rollers in Fig. S1. The polysterene (PS) colloid solution is flown in a one-centimeter wide channel made of double sided tape. The thickness of the adhesive film (dark grey) sets the gap between the two electrodes: 110 $\mu$m. Both the rectangular chamber and the cylindrical obstacles are made of an insulating resin (blue color). The pattern is achieved using conventional UV lithography. The obstacles are located at random positions with possible overlap as seen in the close-up picture of a colloid-free channel. The thickness of the insulating resin is about 2 $\mu$m. The diameters of the colloids and of the obstacles are respectively 4.8 $\mu$m and 10 $\mu$m. Due to the local perturbation to the orientation and magnitude of the electric field in the vicinity of the insulating walls and obstacles, the colloids are electrostatically repelled from the regions covered by the resin patterns.

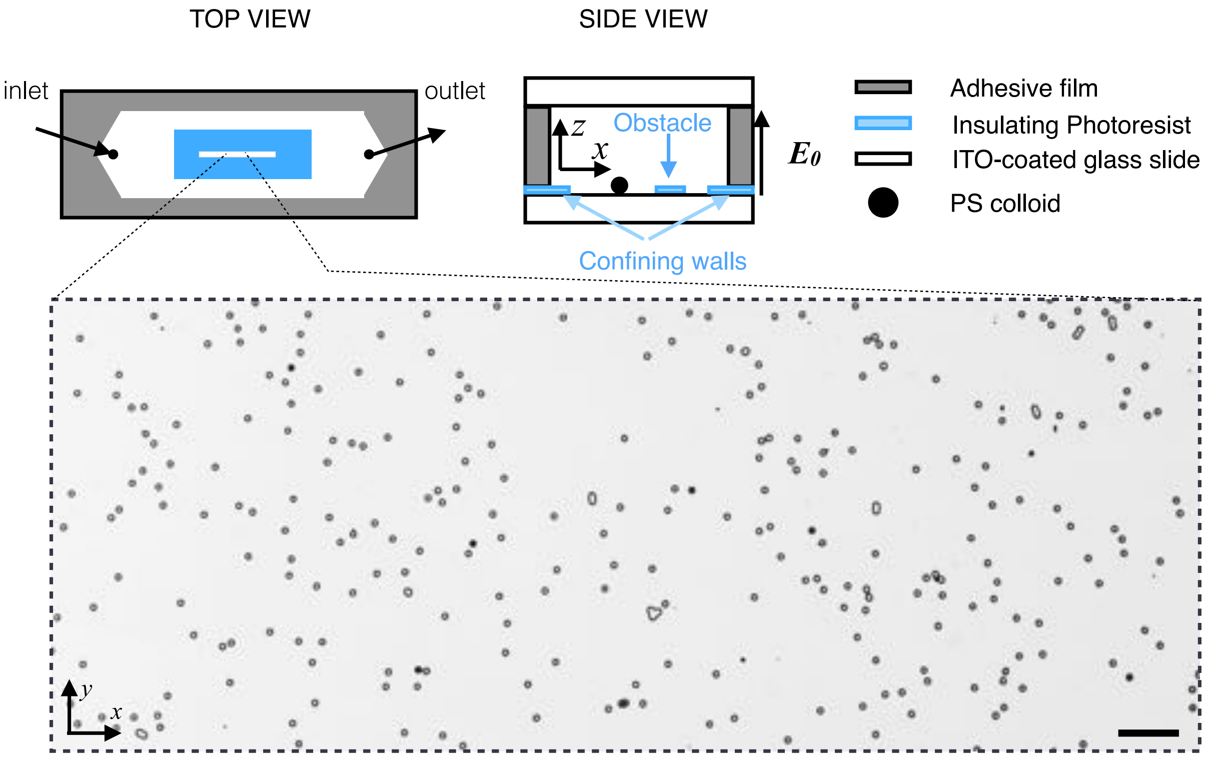


**Figure S1 | Sketch of the microfluidic device. Top view.** A one-centimeter wide channel is used to flow the colloidal solution. The rectangular chamber is delimited by an insulating lithographied resin, and includes cylindrical obstacles of radius 5 microns on the bottom ITO-coated glass slide. The picture of a colloid-free device shows a typical distribution of obstacles. Scale bar: 100 $\mu$m. **Side view.** The colloids roll on the bottom electrode, the obstacles electrostatically repel the approaching rollers. An adhesive film (double-sided scotch tape) sets the gap between the electrodes.

# 2 Supplementary Note 1: Flocking-through-disorder experiments

## 2.1 Global flock morphology: current, density and polarization fields

A flock, by definition, corresponds to a region of space where orientational order exists. The amplitude of a flock, and its extent along the propagation direction, can be measured from three different observables: the local current $J_x(\mathbf{r},t)$ introduced in the main text, the local packing fraction of rollers $\rho(\mathbf{r},t)$, and the local polarization field $\Pi(\mathbf{r},t)$ defined as $J_x(\mathbf{r},t) \equiv v_0\rho(\mathbf{r},t)\Pi(\mathbf{r},t)$. $\Pi$ quantifies the local amount of orientational order regardless of the local area fraction of rollers $\rho(\mathbf{r},t)$. As shown in Fig. S2 their time variations averaged over the channel width convey the same information about the flock morphologies. More quantitatively, the flock length, and the maximal amplitude measured from these three observables are plotted versus $\phi_o$ in Fig. S2. The trends are perfectly consistent. The discontinuity of the amplitude drop at $\phi_o^\star$ is even extremely pronounced for the polarization variable.

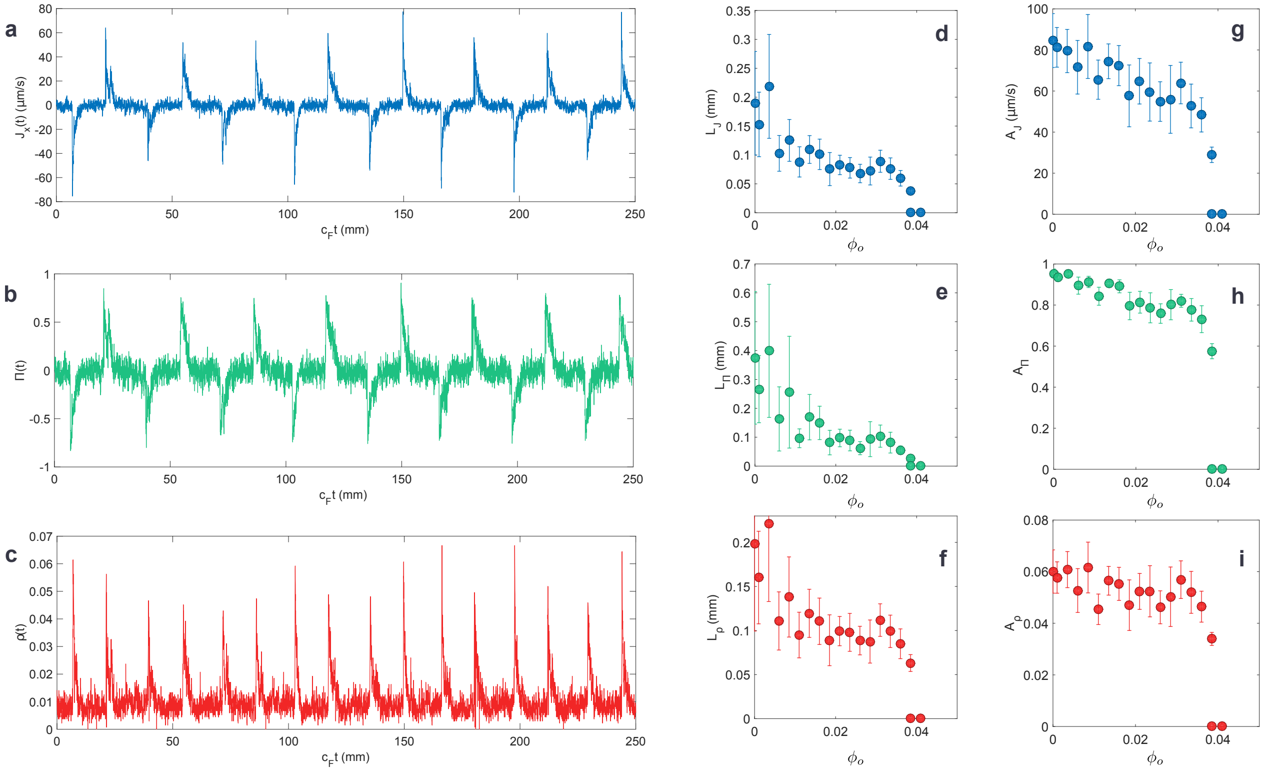


**Figure S2 | Three different probes of orientational order: current, polarization and density.** **a**, Time variations of the local current averaged over the microfluidic-channel width. Note that the distance between two subsequent peaks is not a constant as the observation window is not perfectly centered on the microfluidic channel. **b**, Time variations of the local polarization averaged over the microfluidic-channel width. **c**, Time variations of the local roller density averaged over the microfluidic-channel width. **d**, Flock length measured from the current signal as defined in the main text plotted versus the obstacle fraction. **e**, Same plot for the flock length measured from the polarization signal. **f**, Same plot for the flock length measured from the density signal. **g**, Flock-current amplitude plotted versus the obstacle fraction. **h**, Same plot for the flock-polarization amplitude. **h**, Same plot for the flock-density amplitude.

## 2.2 Isotropy of the current field above $\phi_o^\star$

Above $\phi_o^\star$, by definition, all the global order parameters quantifying orientational order vanish. However, the rollers do not merely form an uncorrelated gaz phase. As emphasized in the main text, collective motion locally persists along extended yet finite paths. However these paths do not allow any macroscopic transport as they are isotropically oriented and only have a finite life time. The global isotropy of the current in this disordered regime is demonstrated in Fig. S3. In Figs. S3a and S3b, we first recall the typical morphology of the flock-current field below and above $\phi_o^\star$. Above $\phi_o^\star$, $\mathbf{J}_{\text{flock}}$ is defined as $\mathbf{J}_{\text{flock}}(\mathbf{r}) = \langle \mathbf{J}(\mathbf{r}, t)\rangle_{t\in\Delta t_F}$, where the time interval $\Delta t_F$ is kept equal to that measured at $\phi_o^\star$. In Figs. S3c and S3d, we plot the flock-current correlation function: $\langle \mathbf{J}_{\text{flock}}(\mathbf{r}') \cdot \mathbf{J}_{\text{flock}}(\mathbf{r}' + \mathbf{r})\rangle_{\mathbf{r}'}$. Whereas they are clearly anisotropic in the flocking regime, all orientational features are lost in the high-disorder limit.

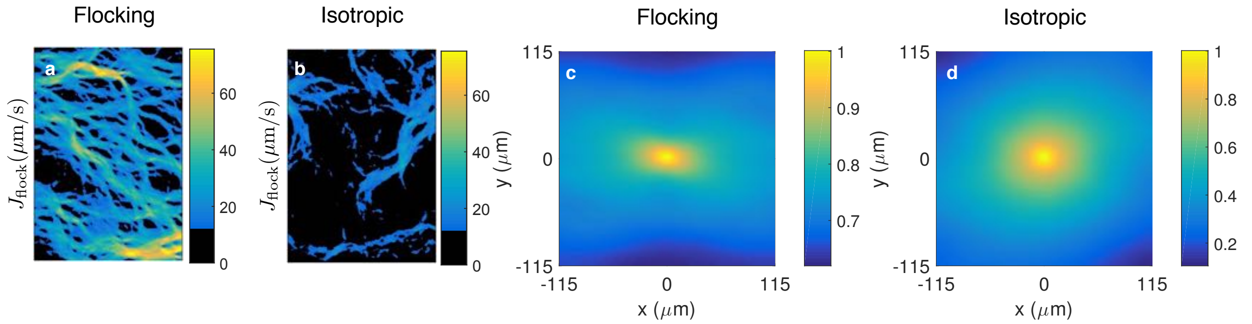


**Figure S3 | Current isotropy above $\phi_o^\star$.** **a**, Magnitude of the flock current $J_{\text{flock}}$ corresponding to $\phi_o/\phi_o^\star = 0.9$. Spatial coarse graining over $12.5\,\mu$m $\times$ $12.5\,\mu$m bins. **b**, Magnitude of the flock current $J_{\text{flock}}$ corresponding to $\phi_o/\phi_o^\star = 1.1$. Spatial coarse graining over $12.5\,\mu$m $\times$ $12.5\,\mu$m bins. The current is averaged over the same time interval as in **a**. **c**, Spatial decay of the normalized flock-current correlations for $\phi_o/\phi_o^\star = 0.9$. The current correlations are anisotropic. **d**, Spatial decay of the normalized flock-current correlations for $\phi_o/\phi_o^\star = 1.1$. The current correlations are isotropic.

## 2.3 Obstacle-Roller Scattering and Effective Diffusion

Fig. S4a shows six scattering diagrams corresponding to six different electric-field amplitudes. The scattering angle is plotted versus the impact parameter $b$ normalized by the obstacle radius $a$, as defined in Fig. 4a in the main document. The range of the obstacle-roller interaction is defined as the value of the impact parameter where the scattering angle vanishes. This range hardly depends on the field magnitude. However, repeating the same experiments with obstacle of increasing size, we find that the repulsion range is proportional to the obstacle radius, Fig. S4b.

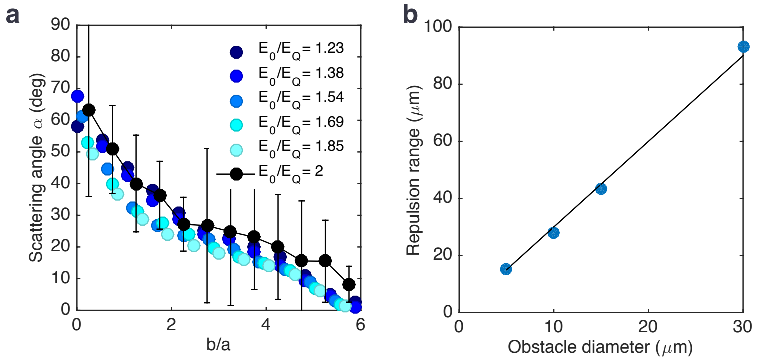


**Figure S4 | Single-roller scattering. a**, Scattering angle plotted as a function of the normalized impact parameter for six different field amplitudes. Error bars: 1sd, shown only for $E_0/E_{\rm Q} = 2$ for sake of clarity. **b**, Circles: repulsion range plotted as a function of the obstacle diameter. Solid line: straight line of slope 3.

# 3 Supplementary Note 2: Flocking-through-disorder theory

## 3.1 Equations of motion of interacting colloidal rollers in a homogeneous media

Starting from the Stokes and Maxwell equations, we established in [34] the equations of motion of colloidal particles propelled by the Quincke mechanism. After lengthy algebra, they can be recast into a compact form. The rollers propel at a constant speed, undergo rotational diffusion with a diffusivity $D$, and interact via effective torques deriving from the angular potential $\mathcal{H}(\mathbf{r}; \hat{\mathbf{p}}_i, \hat{\mathbf{p}}_j)$:

$$\partial_t \mathbf{r}_i(t) = v_0 \hat{\mathbf{p}}_i, \tag{1}$$

$$\partial_t \theta_i(t) = -\partial_{\theta_i} \sum_{j \neq i} \mathcal{H}(\mathbf{r}_i - \mathbf{r}_j; \hat{\mathbf{p}}_i, \hat{\mathbf{p}}_j) + \sqrt{2D}\xi_i(t), \tag{2}$$

where $\mathbf{r}_i(t)$ and $\hat{\mathbf{p}}_i(t) = (\cos\theta_i(t), \sin\theta_i(t))$ are respectively the position and the orientation of the $i^{\rm th}$ roller. The $\xi_i(t)$s are delta-correlated Gaussian white noises of unit variance, and the effective interaction reads:

$$\mathcal{H}(\mathbf{r}; \hat{\mathbf{p}}_i, \hat{\mathbf{p}}_j) = A(r)\hat{\mathbf{p}}_i \cdot \hat{\mathbf{p}}_j + B(r)\hat{\mathbf{p}}_i \cdot \mathbf{r} + C(r)\hat{\mathbf{p}}_j \cdot (2\mathbf{rr} - \mathbb{I}) \cdot \hat{\mathbf{p}}_i. \tag{3}$$

$A(r)$, $B(r)$ and $C(r)$ decay exponentially over a distance $H$ of the order of the microfludic-channel height. They all have the same functional form: $X(\mathbf{r}) = \tau_X^{-1} r^{-n_X} \exp(-r/H)$, with $X = A$, $B$, $C$ and $n_X > 3$. The characteristic relaxation times $\tau_X$ are all of the order $\sim a/v_o$ where $a$ is the colloid radius. Their quantitative expressions and the estimate of their strengths are provided in [34, 35]. We neglect here an additional genuinely long-range interaction associated with a very small coupling constant and which plays no role in the following discussions given the system sizes we consider.

The three terms of the effective potential are *not* specific to colloidal rollers, rather they correspond to the first terms of a systematic multipolar expansion of any effective-interaction potential [36]. The physical meaning of these three terms is clear: $A(r)$ quantifies the strength of the polar interaction promoting the alignment of the roller velocities. This interaction stems from hydrodynamic and electrostatic interactions as well. $B(r)$ corresponds to repulsive interactions. This term is minimized when the direction of the roller $i$ points in the direction opposite to $\mathbf{r}_j - \mathbf{r}_i$. This interaction stems from electrostatics. $C(r)$ combines both hydrodynamic and electrostatic contributions. This third term indicates that the roller $i$ is also prone to align its velocity with a dipolar field centered on the roller $j$.

## 3.2 Roller-obstacle interactions

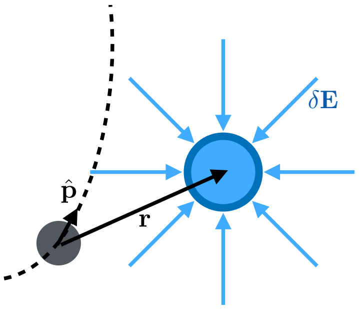


**Figure S5 | Single-roller scattering.** Sketch of a roller (small grey disc) interacting with an obstacle (large blue disc). Dotted line: trajectory. $\delta\mathbf{E}$: in-plane component of the electric field perturbation.

Let us now consider an insulating circular post located at $\mathbf{r} = 0$. This dielectric material deforms the external electric field $\mathbf{E} = E_0\hat{\mathbf{z}}$ used to trigger the Quincke rotation of the colloids. The calculation of the electric-field disturbance induced by a dielectric immersed in a conducting fluid is provided in [34]. Regardless of its specific form, we know that the range of the perturbation is screened over a scale comparable to the distance $H$ between the two electrodes. In addition the obstacle being axisymmetric the perturbation must be radial in the $xy$-plane, and point toward the center of the dielectric obstacle lithographed on the positive electrode, Fig. S5.

An effective torque of the form $\partial_\theta(\hat{\mathbf{p}} \cdot \mathbf{E})$ aligns the roller orientation in the direction opposite to the $xy$-components of the electric field. Therefore the equations of motion of an isolated roller interacting with

a cylindrical obstacle are:

$$\partial_t \mathbf{r}(t) = v_0 \hat{\mathbf{p}}, \tag{4}$$

$$\partial_t \theta(t) = -\partial_\theta \mathcal{H}_\mathrm{o}(\mathbf{r}; \hat{\mathbf{p}}), \tag{5}$$

where the effective repulsion potential has the same form as the roller-roller repulsion:

$$\mathcal{H}_\mathrm{o}(\mathbf{r}; \hat{\mathbf{p}}) = B_\mathrm{o}(r) \hat{\mathbf{p}} \cdot \mathbf{r}. \tag{6}$$

$B_\mathrm{o}(r)$ has the same form as $B(r)$ defined in the previous section: $B_\mathrm{o}(r) \sim \exp(-r/H)/r^4$. The above equations are of course complemented by a hard-core repulsive interaction between the rollers and the insulating post.

## 3.3 Flocking transition in weak quenched disorder

### 3.3.1 Kinetic theory

We first outline how to construct the hydrodynamic equations ruling the temporal evolution of the density and current fields in the presence of a dilute ensemble of weak scatterers. We use here a conventional kinetic-theory framework reviewed e.g. in [37]. We first write a conservation equation for the one-point distribution $\psi(\mathbf{r}, \theta, t)$, i.e. the probability to find a particle at position $\mathbf{r}$ with an orientation $\hat{\mathbf{p}} = (\cos\theta, \sin\theta)$:

$$\partial_t \psi(\mathbf{r}, \theta, t) + v_0 \hat{\mathbf{p}} \cdot \nabla \psi(\mathbf{r}, \theta, t) - D \partial_\theta^2 \psi(\mathbf{r}, \theta, t) = -\partial_\theta \mathcal{J}_\mathrm{int}(\mathbf{r}, \theta, t) + \mathcal{S}_\mathrm{o}(\mathbf{r}, \theta, t) \tag{7}$$

For interaction-free particles moving in a homogeneous media, the r.h.s of the above equation vanishes and $\psi$ is merely advected due to self-propulsion, and diffuses in the $\theta$ direction due to the angular noise acting on the rollers' direction. The angular current $\mathcal{J}_\mathrm{int}$, and $\mathcal{S}_\mathrm{o}(\mathbf{r}, \theta, t)$ account for the roller-roller and the roller-obstacle interactions respectively. Starting from the microscopic equations Eqs. (1),(2) and (3), we derived the functional form of $\mathcal{J}_\mathrm{int}(\mathbf{r}, \theta, t)$ in [34]. Briefly, as the range of the effective potential $\mathcal{H}$ is of the order of 40 colloid radii, in a homogeneous isotropic phase, each colloid interacts on average with $\sim 20$ neighbors. This large number is even a decade larger when a flock forms, which suggests using a mean field description to establish the functional form of $\mathcal{J}_\mathrm{int}$. More precisely, assuming that the two points correlation function factorizes: $\psi^{(2)}(\mathbf{r}, \hat{\mathbf{p}}; \mathbf{r}', \hat{\mathbf{p}}') = \psi(\mathbf{r}, \hat{\mathbf{p}})\psi(\mathbf{r}', \hat{\mathbf{p}}')$ and vanishes for $|\mathbf{r} - \mathbf{r}'| < 2a$ (to account for the finite size of the rollers), $\mathcal{J}_\mathrm{int}$takes the form:

$$\mathcal{J}_\mathrm{int} = -\psi(\mathbf{r}, \theta) \int_{|\mathbf{r}-\mathbf{r}'|>2a} \mathrm{d}\theta' \mathrm{d}\mathbf{r}' \psi(\mathbf{r}', \hat{\mathbf{p}}') \partial_\theta \mathcal{H}(\mathbf{r} - \mathbf{r}'; \theta, \theta') \tag{8}$$

Two different approximations are used to compute the $\mathcal{S}_\mathrm{o}$ term in Eq. (7). Let us first ignore the specifics of the roller obstacle interactions, and consider a simplified description of the scattering process. Following [38], we focus first on the asymptotic limit of an infinitely dilute ensemble of uncorrelated scatterers, and use a Boltzmann-like approximation. We make the molecular chaos hypothesis and restrain ourselves to binary collisions. Within this framework, at large scales, scattering can be described without loss of generality as a change in the orientation $\theta$ by an increment $\pm\epsilon$ upon collision. Provided that the persistence length of a free roller exceeds the typical inter-obstacle distance, which is the case in our experiments, collisions occur at a rate $2v_0\phi_\mathrm{o}a/(\pi a_o^2)$ which yields in the small-$\epsilon$ limit:

$$\mathcal{S}_\mathrm{o} = (D'\phi_\mathrm{o}) \partial_\theta^2 \psi(\mathbf{r}, \theta, t), \tag{9}$$

where $D' = \frac{1}{2} v_0 a \epsilon^2/(\pi a_o^2)$. The obstacle interactions renormalize the angular diffusivity of the particle which increases in an affine fashion with $\phi_\mathrm{o}$ in agreement with our experimental findings in the isotropic phases:

$$D(\phi_\mathrm{o}) = D + D'\phi_\mathrm{o} \tag{10}$$

At large scales, the particle motility converts the collisions with a quenched ensemble of scatterers into a time-dependent angular noise. This scenario is the exact analogous of that observed in a dilute Lorentz gaz where ballistic particles undergo elastic collisions on fixed scatterers.

Given the mean-field description for the roller interactions, and the Boltzmann description of the obstacle scattering, the two types of interactions decouple in Eq. (7). Consequently, Eqs. (7), (8), and (9) suggest that the emergence, and suppression, of collective motion in dilute disordered media should belong to the same first-order universality class as the Vicsek transition between a gas and an orientationally ordered state. We recall that the seminal Vicsek model concerns a 2D ensemble of motile spins interacting via ferromagnetic

interactions competing with a time-dependent angular noise [39, 40]. Upon decreasing the noise amplitude, the spins undergo a *first order* transition from an isotropic to a polar state, see e.g. [40, 41] and references therein. The first order nature of the transition arises from the nucleation and subsequent steady propagation of nonlinear band-like excitations akin to the colloidal flocks reported in this letter. The global suppression of polar order found in our experiments is therefore strongly expected to be triggered by the increase of rotational diffusion resulting from random scattering processes. We further confirm this hypothesis below, by constructing a hydrodynamic description of the roller flocks cruising through disorder.

#### 3.3.2 Hydrodynamic theory

In order to confirm the relevance of our main hypothesis, namely the Boltzmann approximation to account for interaction with the random scatterers, we first derive the equations of motion of the hydrodynamic variables $\rho(\mathbf{r},t) \equiv \int \psi(\mathbf{r},\theta)\,\mathrm{d}\theta$ and $\mathbf{J}(\mathbf{r},t) \equiv \int \hat{\mathbf{p}}(\theta)\,\psi(\mathbf{r},\theta)\mathrm{d}\theta$ close to an isotropic state. Within this hydrodynamic framework we are able to make a quantitative prediction regarding the extent of the flocking patterns and to compare them to our experimental findings.

We complement mass conservation:

$$\partial_t \rho(\mathbf{r},t) + \nabla\cdot\mathbf{J}(\mathbf{r},t) = 0, \tag{11}$$

by the time evolution of the current field. Multiplying Eq. (7) by $\hat{\mathbf{p}}$, averaging over $\psi$ and keeping only the leading order terms in a gradient expansion yields a relation between $\rho$, $\mathbf{J}$ and the local nematic tensor $\mathbf{Q}$, defined as: $\rho\mathbf{Q} = \langle\hat{\mathbf{p}}\hat{\mathbf{p}} - \frac{1}{2}\mathbb{I}\rangle$, see [34] for more technical details, or [37]:

$$\partial_t\mathbf{J} + v_0^2\nabla\cdot\left[\rho\left(\mathbf{Q}+\frac{1}{2}\mathbb{I}\right)\right] = -D(\phi_o)\mathbf{J} + \alpha_1\rho(\mathbb{I}-2\mathbf{Q})\cdot\mathbf{J} - \beta\frac{v_0}{2}(\mathbb{I}-2\mathbf{Q})\cdot\rho\nabla\rho \tag{12}$$

where $\alpha_1$ and $\beta$ are hydrodynamic coefficients defined by the spatial averages of $A(r)$ and $B(r)$, defined in Eq. (3). A self-consistent hydrodynamic description of the polar active fluid, requires expressing the local nematic tensor as a function of $\rho$ and $\mathbf{J}$. As we are here interested in describing the onset of collective motion, we use a closure relation valid close to an isotropic state. Following the approach reviewed in [42] we write down a dynamical equation for the $\mathbf{Q}$ field, ignore its temporal variations, discard higher order angular multipoles of the distribution function and consistently restrain ourselves to the lowest order gradient terms. We are then left with a generic form akin to the Toner and Tu equation originally inferred from symmetry considerations [43]:

$$\begin{aligned}\partial_t\mathbf{J} + \frac{3\alpha_1}{8D(\phi_o)}\mathbf{J}\cdot\nabla\mathbf{J} = &\left[\alpha_1\rho - D(\phi_o) - \frac{\alpha_1^2}{2v_0^2 D(\phi_o)}J^2\right]\mathbf{J} - \frac{v_0}{2}\left(v_0+\beta\rho\right)\nabla\rho \\ &- \frac{5\alpha_1}{8D(\phi_o)}(\nabla\cdot\mathbf{J})\mathbf{J} + \frac{5\alpha_1}{16D(\phi_o)}\nabla(J^2) + \frac{\alpha_1\beta}{2v_0 D(\phi_o)}(\nabla\rho\cdot\mathbf{J})\mathbf{J} + O(\nabla^2)\end{aligned} \tag{13}$$

We shall stress that all the hydrodynamic coefficients are computed from the microscopic equation of motion and can be quantitatively measured, or estimated, from our experiments [35]. This equation is the analogous of that derived in [34], replacing the bare rotational diffusivity $D$, by $D(\phi_o) = D + D'\phi_o$.

#### 3.3.3 Flock morphologies

In order to compute the shape of the colloidal flocks we look for localized solutions of Eqs. (11) and (13) which are homogeneous along the $y$-direction and steadily propagate along the $x$-direction with a velocity $c$: $\mathbf{J}(\mathbf{r},t) = J(x-ct)\hat{\mathbf{x}}$, $\rho(\mathbf{r},t) = \rho(x-ct)$. By doing so, mass conservation, Eq. (11), takes the form of a local relation between $\rho$ and $\mathbf{J}$

$$\rho(z) = \rho_\infty + \frac{\mathbf{J}(z)}{c} \tag{14}$$

where $z = x - ct$, and $\rho_\infty$ is the fraction of active particles in the isotropic region away from the flock. Similarly, (13) reduces to a non-linear ordinary differential equation:

$$\mathcal{D}[J]\ddot{J}(z) + \mathcal{F}[J]\dot{J}(z) + \mathcal{H}[J]J(z) = 0, \tag{15}$$

where

$$\mathcal{H}[J] = [\alpha_1\rho_\infty - D(\phi_o)] + \frac{\alpha_1}{c}J - \frac{\alpha_1^2}{2v_0 D(\phi_o)}J^2, \tag{16}$$

$$\mathcal{F}[J] = \left[c - \frac{v_0}{2c}\left(v_0+\beta\rho_\infty\right)\right] - \left[\frac{3\alpha_1}{8D(\phi_o)} + \frac{v_0\beta}{2c^2}\right]J + \frac{\alpha_1\beta}{2v_0 c D(\phi_o)}J^2. \tag{17}$$

The second-order term $\mathcal{D}[J]\ddot{J}(z)$ comes from the $\mathcal{O}(\nabla^2)$ terms in Eq. (13), it has a lengthy expression which we do not report here as it is useless to compute the flock length.

Eq. (15) can be readily written in the form of a dynamical system, and describing the shape of propagating patterns amounts to describe the cycles of this dynamical system, i.e. the periodic solutions of (15). We showed in [44, 45] that homoclinic cycles correspond to solitonic band-shape flocks. The typical extent of these localized excitations is estimated by looking at the linear stability of Eq. (15) around a homogeneous and isotropic state ($J(z) = 0$). As first pointed out in [46], when propagating solutions exist the resulting linear system has one stable and one unstable eigenvalues corresponding respectively to the width of the flock front, and to the extent of its long tail which is a good approximation of the flock length $L_{\rm F}$, see Fig. S2. In the weakly polarized tail the second-order term in Eq. (15) remains much smaller than the two others, consistently with the quasi isotropic approximation used to derive Eq. (13). Therefore, after straightforward algebra, discarding subdominant corrections in $\mathcal{D}[0]$, we predict the relation:

$$L_{\rm F} = \frac{v_0}{\alpha_1}\left[\frac{\frac{c}{v_0} - \frac{v_0}{2c}\left(1 + \frac{\beta\rho_\infty}{v_0}\right)}{\rho_{\rm c}(\phi_{\rm o}) - \rho_\infty}\right], \tag{18}$$

where $\rho_{\rm c}(\phi_{\rm o}) = (D + D'\phi_{\rm o})/\alpha_1$. The above equation relates the flock length, $L_{\rm F}$, the area fraction in the surrounding gaz phase, $\rho_\infty$, the strength of the roller repulsion, $\beta$, and of the alignment terms, $\alpha_1$ at the hydrodynamic level. $\rho_{\rm c}(\phi_{\rm o})$ compares the strength of the alignment interactions to the angular diffusion which impedes orientational order. It corresponds to the roller fraction above which Eq. (13) would predict a mean-field transition toward collective motion (i.e. ignoring all the gradient terms). Eq. (18) indicates that the macroscopic band length results from the amplification of the microscopic length scale $v_0/\alpha_1$ (of the order of the colloid size) by a factor $[\rho_{\rm c}(\phi_{\rm o}) - \rho_\infty]^{-1}$ which can be arbitrarily large as the roller fraction in the gas approaches $\rho_{\rm c}$.

In order to test this prediction, we measure: (i) $c$ which is equal to $v_0$ in all our experiments, Fig. 2a. (ii) $D'$ from the slope of the linear increase of $D$ with $\phi_{\rm o}$ in Fig. 4d, and (iii) the density $\rho_\infty$ in the isotropic phase through which the flocks propagate. In addition, in [35], we measured the value of $\alpha_1$ from the continuous bifurcation from a gas to a vortex state in circular confinements, and found $\alpha_1 = 3 \times 10^{-3}\,{\rm s}^{-1}$. We are hence left with the theoretical prediction with no free fitting parameter. In Fig. 2.c, which we reproduce below, we find an excellent agreement with our experimental measurements.

Given the number of simplifications needed to derive the hydrodynamic model, this agreement confirms the robustness of our results, and our main conclusion: the emergence and suppression of collective motion induced by a dilute ensemble of obstacles is a genuine non-equilibrium first order transition. This transition falls in the same universality class as the flocking transition of the Vicsek type.

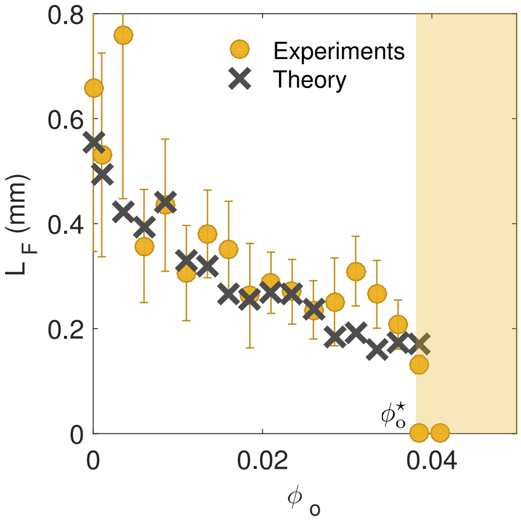


**Figure S6 | Variations of the flock length with the obstacle fraction.** Comparison of the measured flock length to the theoretical prediction given by Eq. (18).

## 3.4 Emergence of flowing-channel networks

The theory introduced in the previous section is unable to capture the inner structure of the colloidal flocks. The sole spatial feature of disorder included in this $0^{\text{th}}$ order model is the mean obstacle fraction. However, Eq. (13) could be modified to account for the spatial heterogeneities of the obstacle distribution by replacing $\phi_{\text{o}}$ by its local value $\phi_{\text{o}}(\mathbf{r})$ defined at a scale much larger than the typical inter-obstacle distance. This modified model would endow the rollers with a higher rotational diffusivity, hence a smaller translational diffusivity, in the regions where the obstacle density is large. A direct consequence would be the accumulation of the colloids in the regions where the obstacles are the most concentrated. This prediction is in total contradiction with our experimental observations. In order to go beyond this oversimplified picture, we need to more accurately account for the impact of the spatial heterogeneity of disorder.

### 3.4.1 Hydrodynamics of a strongly polarized flock of rollers: homogeneous media

A major limitation of the current kinetic theories of polar active matter is that they fail in providing a unified hydrodynamic description valid at all densities and polarizations. As a matter of fact they all rely on closure approximations which are either valid in the weakly polarized or, conversely, in the strongly polarized limit. As we now aim at describing the spatial structure of the flock front which is strongly polarized, Fig. **S2**, we use a closure relation which is different from that used in the previous section to model nearly isotropic states. We neglect the possible local melting of orientational order and solely focus on the orientational fluctuations of the polarization field $\mathbf{\Pi} = \mathbf{J}/(v_0\rho)$ close to the head of the flock. In fact, we make the following ansatz for the one-point function $\psi(\mathbf{r},\theta,t) = \rho(\mathbf{r},t)\delta(\hat{\mathbf{p}} - \mathbf{\Pi}(\mathbf{r},t))$. This ansatz implies that $\mathbf{Q} = \mathbf{\Pi\Pi} - \frac{1}{2}\mathbb{I}$, and the hydrodynamic equation Eq. (12) takes a simple form at leading order in a gradient expansion:

$$\partial_t \mathbf{\Pi} + v_0 \mathbf{\Pi}\cdot\nabla\mathbf{\Pi} = \mathbb{P}\cdot\left[-\beta\nabla\rho + \alpha_2\nabla^2(\rho\mathbf{\Pi}) + \gamma\tilde{\Delta}\cdot(\rho\mathbf{\Pi})\right] \tag{19}$$

where the projection operator $\mathbb{P} = \mathbb{I} - \mathbf{\Pi\Pi}$ constrains the modulus of $\mathbf{\Pi}$ to be a constant, and

$$\tilde{\Delta} = \begin{pmatrix} \partial_{xx} - \partial_{yy} & 2\partial_{xy} \\ 2\partial_{xy} & \partial_{yy} - \partial_{xx} \end{pmatrix}. \tag{20}$$

All the terms in Eq. (19) have a clear physical meaning. The l.h.s is the convective derivative of the polarization which is advected due to self-propulsion. The first term on the r.h.s is a pressure term. $\beta\nabla\rho$ results from the repulsive interactions between the rollers. Finally, the two positive hydrodynamic coefficients $\alpha_2$ and $\gamma$ measure the (anisotropic) stiffness of this broken symmetry fluid. $\alpha_2$ stems from the alignment interactions, whereas $\gamma$ derives from the dipolar term in Eq. (3). This equation is a simplified version of the hydrodynamic theory provided in [34] where weak local melting was allowed. It is reminiscent of the Toner and Tu theory in the strongly polarized limit yet it includes an additional anisotropic term. We show below that the emergent network of preferred flowing routes is not specific to this anisotropic addition, and is therefore expected to be a robust large-scale feature of any polar liquid flowing through repelling obstacles.

### 3.4.2 Hydrodynamics of a strongly polarized flock of rollers: heterogeneous media

We now generalize Eq. (19) to include the effect of disorder. We here model disorder within another asymptotic approximation. In the same spirit as our roller-roller interaction theory, in the limit of high obstacle density we provide a mean-field description of the $\mathcal{S}_{\text{o}}$ term in Eq. (7) and write it as $\mathcal{S}_{\text{o}} \equiv -\partial_\theta \mathcal{J}_{\text{o}}(\mathbf{r},\theta,t)$, where the angular current $\mathcal{J}_{\text{o}}$ results from the angular advection of the probability density $\psi(\mathbf{r},\theta,t)$ by the repulsive torques defined in Eq. (5). The net torque felt by a roller at $\mathbf{r}$ and oriented along $\theta$ is $\int \phi_o(\mathbf{r}')\partial_\theta\mathcal{H}_{\text{o}}(\mathbf{r}-\mathbf{r}';\theta)\mathrm{d}\mathbf{r}'$, where we $\phi_{\text{o}}(\mathbf{r})$ is the local packing fraction of obstacles. The resulting current is:

$$\mathcal{J}_{\text{o}} = -\psi(\mathbf{r},\theta)\int \mathrm{d}\mathbf{r}'\phi_o(\mathbf{r}')\partial_\theta\mathcal{H}_{\text{o}}(\mathbf{r}-\mathbf{r}';\theta) \tag{21}$$

We then follow the same procedure as in the previous section and establish the hydrodynamic equation of the polarization field. We multiply Eq. (7) by $\hat{\mathbf{p}}$, and integrate it over $\theta$ using the polar closure ansatz: $\psi(\mathbf{r},\theta,t) = \rho(\mathbf{r},t)\delta(\hat{\mathbf{p}} - \mathbf{\Pi}(\mathbf{r},t))$ and obtain:

$$\partial_t \mathbf{\Pi} + v_0 \mathbf{\Pi}\cdot\nabla\mathbf{\Pi} = \mathbb{P}\cdot\left[-\beta\nabla\rho + \alpha_2\nabla^2(\rho\mathbf{\Pi}) + \gamma\tilde{\Delta}\cdot(\rho\mathbf{\Pi}) + \mathbf{F}_{\text{o}}\right]. \tag{22}$$

The only modification to Eq. (19) is the additional random-force term $\mathbf{F}_{\text{o}}$ which accounts for the coupling of the polar fluid to disorder. Remarkably this random-force field derives from a potential: the local obstacle density.

$$\mathbf{F}_{\text{o}}(\mathbf{r}) = -\beta_{\text{o}}\nabla\phi_{\text{o}}, \tag{23}$$

where $\beta_{\text{o}}$ is a positive constant which quantifies the strength or the repelling torque. For a uniform set of spatially uncorrelated obstacles, $\mathbf{F}_{\text{o}}(\mathbf{r})$ is a quenched random field of zero mean and variance:

$$\overline{\mathbf{F}_{\text{o}}(\mathbf{r})\mathbf{F}_{\text{o}}(\mathbf{r'})} = \beta_{\text{o}}^2\phi_{\text{o}}\nabla\nabla\delta(\mathbf{r}-\mathbf{r'}), \tag{24}$$

where $\overline{X}$ denotes the average over disorder of the $X$ observable.

This term has also a very clear physical meaning: $\mathbf{F}_{\text{o}}$ focalizes the polar liquid in the valleys of the potential defined by $\phi_{\text{o}}$. We elucidate below how the pressure arising from the roller repulsion and the effective elasticity stemming from the alignment interactions compete with disorder to set the spatial structure of this polar liquid.

### 3.4.3 Response to a quenched random field and formation of sparse river networks

The full analytical description of an active fluid randomly stirred by quenched disorder goes far beyond the scope of this article. However a clear physical insight can be gained from a linearized theory. Let us compute the linear response of the density and polarization fields to a static perturbation $\mathbf{F}_{\text{o}}$. The unperturbed state is assumed to be homogeneously flowing along the $\hat{\mathbf{x}}$ direction. We introduce the angular deviation $\delta\theta(\mathbf{r})$ defined as $\mathbf{\Pi}(\mathbf{r}) = \hat{\mathbf{x}} + \delta\theta(\mathbf{r})\hat{\mathbf{y}} + \mathcal{O}(\delta\theta^2)$, and the density perturbation $\rho(\mathbf{r}) = \bar{\rho} + \delta\rho(\mathbf{r})$. The linearized version of the mass-conservation equation and Eq. (19) are:

$$\partial_t\delta\rho + v_0\partial_x\delta\rho + (v_0\bar{\rho})\partial_y\delta\theta = 0, \tag{25}$$

$$\partial_t\delta\theta + v_0\partial_x\delta\theta = -\beta\partial_y\delta\rho + (\alpha_2\bar{\rho})\Delta\delta\theta + (\gamma\bar{\rho})(\partial_{yy}-\partial_{xx})\delta\theta + 2\gamma\partial_{xy}\delta\rho + F^{\perp}, \tag{26}$$

where $F^{\perp} = \mathbf{F}_{\text{o}}\cdot\hat{\mathbf{y}}$ is the component of the random force field in the direction transverse to the mean spontaneous flow. Let us first briefly sketch the stability of this linear system, without going in the details of the calculation which are unimportant to the network formation. The isotropic elasticity ($\alpha_2$ term) stabilizes both the splay and the bend deformations of the polarization field. Conversely the anisotropic contribution ($\gamma$ terms) further stabilizes the splay modes while destabilizing the bend modes. However there always exists a finite range of hydrodynamic coefficients yielding a fully stable dynamics at all wave-lengths provided that $\alpha_2/\gamma < \bar{\rho}$ is sufficiently small. Our estimate from the microscopic parameter values yields $\alpha_2/\gamma \sim 1/10$ [35], which is indeed smaller that the colloid fraction at the flock front. In addition the transverse confinement of the polar flock in a rectangular geometry further suppresses any form of orientational instability. Consistently, we do not observe any sign of spontaneous destruction of polar order, or any density modulation for flock cruising in obstacle-free channels. Therefore, at this stage, we shall focus on the regime where Eqs. (25) and (26) are linearly stable.

As we are interested in the statistics of the *static* structure of the flock, we ignore the transient and readily solve the linear response in Fourier space introducing the Fourier modes $\delta\theta(\mathbf{r}) = \delta\theta_{\mathbf{q}}\exp(i\mathbf{q}\cdot\mathbf{r})$, $\delta\rho(\mathbf{r}) = \delta\rho_{\mathbf{q}}\exp(i\mathbf{q}\cdot\mathbf{r})$, $F^{\perp} = F^{\perp}_{\mathbf{q}}\exp(i\mathbf{q}\cdot\mathbf{r})$. The resulting density and orientational fluctuations are:

$$\overline{|\delta\rho_{\mathbf{q}}|^2} = \frac{\bar{\rho}^2 q_y^2}{\left(v_0 q_x^2 - \beta\bar{\rho}q_y^2\right)^2 + (\alpha_2-\gamma)^2\left(q_x^3 - q_x q_y^2\right)^2}\overline{|F^{\perp}_{\mathbf{q}}|^2} \tag{27}$$

and

$$\overline{|\delta\theta_{\mathbf{q}}|^2} = \frac{q_x^2}{\left(v_0 q_x^2 - \beta\bar{\rho}q_y^2\right)^2 + (\alpha_2-\gamma)^2\left(q_x^3 - q_x q_y^2\right)^2}\overline{|F^{\perp}_{\mathbf{q}}|^2} \tag{28}$$

These equations indicate that the random force field promotes both density and orientational fluctuations. However these fluctuations are hindered by the effective orientational elasticity, the active-fluid pressure and self-propulsion. The consequences of these competitions are very clear when looking at the transverse and quasi longitudinal modes.

(i) **Transverse fluctuations: $\mathbf{q} = q_y\hat{\mathbf{y}}$.** Disorder cannot excite any stationary transverse angular mode (pure splay mode), but yields generic density fluctuations. Using Eqs. (27), and (23) we find:

$$\overline{|\delta\rho_{\mathbf{q}}|^2} = \left(\frac{\beta_{\text{o}}}{\beta}\right)^2\phi_{\text{o}} \tag{29}$$

At all wave-lengths the density fluctuations are set by the competition between the obstacle repulsion which focalizes the rollers in the valley of the potential $\phi_o$ and the inter-roller repulsion that bounds the maximal local density.

(ii) **Longitudinal fluctuations:** $q_x \gg q_y$. The quasi longitudinal modes corresponds to bend excitations of the polarization field. Again, using Eqs. (28), and (23) we find:

$$\overline{|\delta\theta_{\mathbf{q}}|^2} = \frac{\beta_o^2\phi_o}{v_o^2 + q_x^2(\alpha_2-\gamma)^2\bar{\rho}^2}\left(\frac{q_y}{q_x}\right)^2 \tag{30}$$

In the small-$q$ limit the amplitude of the orientational fluctuations is mostly set by the competition between self-propulsion and obstacle repulsion. This scaling translates a simple phenomenon, for a given obstacle strength the magnitude of the angular perturbation is an increasing function of the time spent in the interaction region. As this time decreases linearly with $v_0$, angular fluctuations are obviously expected to decay with $\beta_o/v_0$. The faster the rollers the less time they feel the obstacle repulsion. The second term in the denominator of Eq. (30) has a very different origin, and provides a qualitative explanation for the emergence of sparse river networks. The focalization of the rollers in the valleys of $\phi_o$ is restrained by the bending elasticity of the polar liquid. The higher $\alpha_2$, and the smaller $\gamma$, the stiffer are the bending modes. In addition, as in all broken symmetry fluid, the mode having the smallest wave-lengths are the stiffest. Therefore even though the random force field drives the rollers along its minima, some of its valleys are much more difficult to flow in as they require a strong bend of the flow lines. The higher the obstacle fraction the more tortuous the valleys of $\phi_o(\mathbf{r})$, thereby limiting the number of paths allowed by the bending stiffness of the active fluid. At the linear-response level the angular fluctuations scale with $\phi_o$.

Of course the geometry of a sparse network cannot be quantitatively captured by a mere linear analysis, yet it has allowed us to single out the very mechanisms responsible for their formation.

### 3.5 Disorder-induced melting and emergent river networks: a robust picture

We shall now stress on the robustness of our two main results: (i) the suppression of flocking motion observed in our experiments falls in the same class as the first order Vicsek transition, and (ii) the inner structure of the flocks is that of an increasingly sparse river network. These two results do not rely on any feature specific to colloidal-roller fluids (Quincke propulsion, electrostatic and hydrodynamic interactions, colloidal scale, etc). They apply to *any* polar active material cruising through repelling obstacles.

However, we have focused on situations where the obstacles renormalize the bare diffusivity of isolated rollers. At higher obstacle fraction, or much stronger repulsion, a qualitative change in the dynamic of motile particles occurs: they do not diffuse at long times, but rather undergo sub-diffusive motion due to long-time trappings as reported in [38]. The generalization of our results to this limit goes far beyond the scope of this paper. In this case, both the very nature of the suppression of orientational order together with the existence of genuine long-range orientational order in 2D remains an open question in this regime [47].

## 4 Supplementary Note 3: Flocking through periodic lattices

We close this supplementary not by reporting a series of additionnal experiments conducted in ordered lattices of obstacles, see Supplementary Video 5. The obstacles have the same diameter as in the main text (10 $\mu$m), but form a square lattice with the $(1,1)$ axis parallel to the direction of the main channel, Fig. **S7**a. As in disordered geometries, we find that collective motion is sharply suppressed upon increasing the obstacle fraction $\phi_o$, or decreasing the roller density $\rho$. Irrespective whether the obstacles form a periodic lattice or not, the emergence of collective motion is a first order transition relying on the nucleation and growth of macroscopic band-like excitations. The discontinuity of the transition in both geometries is clearly seen in Fig. **S7**b, which shows how the flock amplitude, $\rho_F$ varies as a function of the mean roller density $\rho$. Interestingly, we observe that flocks are more robust to random obstacles; colloidal flocks are found at smaller densities of colloids in disordered media. This observation is very consistent with a nucleation picture. In a disordered ensemble of obstacles, a flock can nucleate and grow from a region where the obstacle density is locally small. The flock can then propagate through the river network separating the regions of high obstacle density. For the same value of $\phi_o$, no such low-obstacle density region exist in a periodic lattice and no flock is then seen to propagate.

In addition a very strong qualitative difference exist in this ordered geometry. No sparse river network forms. The inner structure and dynamics of the flock remain very homogeneous in the direction transverse to the mean flow, even at the onset of melting, see Fig. **S7**c. The rollers flow through the entire region left around the mere superposition of depleted wakes centered on the obstacle postions. This result is very

consistent with the model introduced in the previous section to account for the emergence of river networks in disordered media. When described at scales larger than the lattice spacing, the obstacle-density field is uniform. Therefore the random stirring term in Eq. (22) vanishes, hence it cannot result in the bending of the roller flow. Conversely, in random media local fluctuations in the obstacle density drive the roller into increasingly sparse and tortuous valleys as $\phi_o$ increases yielding a markedly different geometry of the flock current, see Fig. S7d.

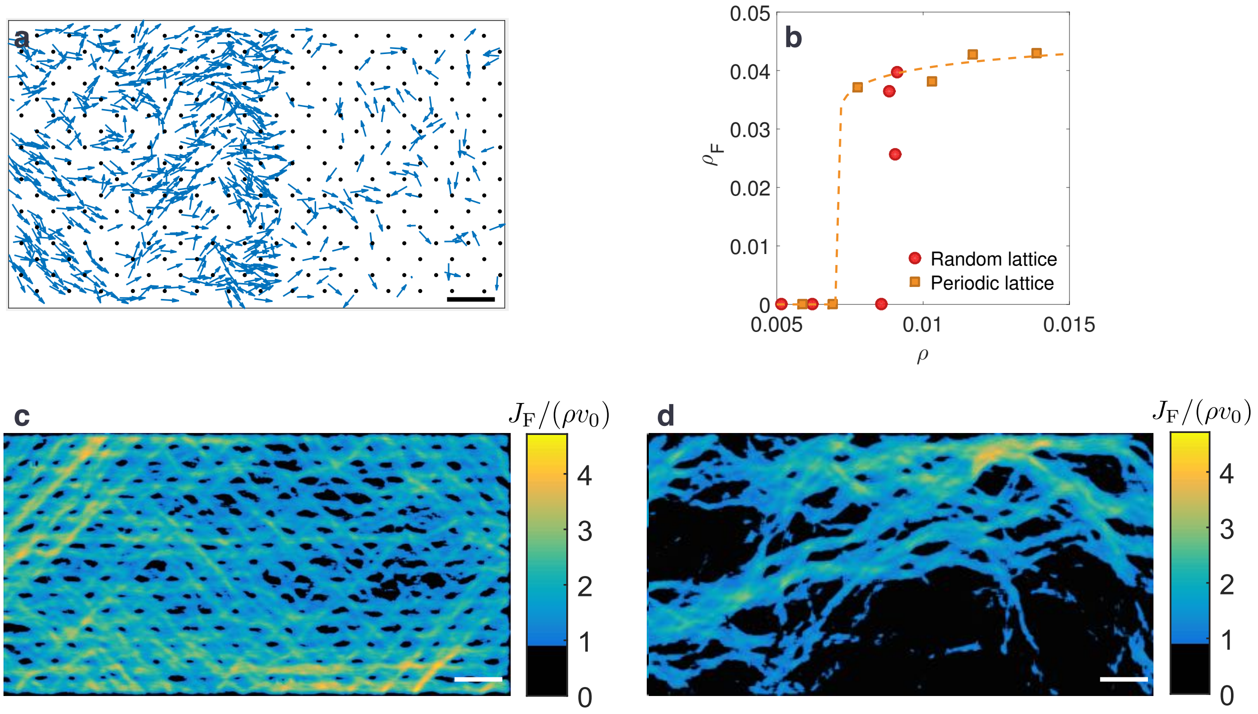


**Figure S7 | Flocking through a periodic lattice of obstacles.** **a**, Close-up on the head of a colloidal swarm propagating past a square lattice of obstacles (black dots). The arrows are located at the colloid positions and point along the orientation of their velocities. Obstacle packing fraction: $\phi_o = 3 \times 10^{-2}$. Scale bar: 100 $\mu$m. **b**, Variations of the amplitude of the flock $\rho_F$ as a function of the mean roller fraction. $\rho_F$ is the difference between the maximal density at the flock front and the density away from the flock in the isotropic phase. See Fig. **S2**. **c**, Map of the normalized flock-current $J_F(\mathbf{r})/(\rho v_0)$ at the onset of melting in a periodic lattice ($\phi_o = 3 \times 10^{-2}$, $\rho = 7.76 \times 10^{-3}$). No sparse network forms. The region where the rollers flow corresponds to the area left by the mere superposition of depleted wakes centered on the obstacle postions. **d**, Comparison with the map of the normalized flock-current $J_F(\mathbf{r})/(\rho v_0)$ at the onset of melting in a random lattice ($\phi_o = 3 \times 10^{-2}$, $\rho = 1.0 \times 10^{-2}$). A river network forms. The geometry of the flowing route is very different from **c**.

# 5 Description of the supplementary videos

1. Supplementary video 1: A colloidal flock emerges from a population of $\sim 9,000$ colloids propelling in a 5mm $\times$ 1mm obstacle-free channel. The flock coexists with a gas phase where all the rollers propel themselves along random directions. Colloid diameter: $4.8\,\mu$m. Field amplitude $E_0 = 2\,\text{V}/\mu\text{m}$.

2. Supplementary video 2: A colloidal-roller flock cruises coherently through a random ensemble of circular obstacles placed in a 15mm $\times$ 1mm rectangular chamber. $\phi_\text{o} = 2 \times 10^{-2}$. The flock coexists with an isotropic phase. Colloid diameter: $4.8\,\mu$m. Obstacle diameter: $10\,\mu$m. Field amplitude $E_0 = 2\,\text{V}/\mu\text{m}$.

3. Supplementary video 3: Colloidal rollers propelling themselves through a random ensemble of circular obstacles placed in a 15mm$\times$1mm rectangular chamber. $\phi_\text{o} = 5\times 10^{-2}$. No large-scale collective motion can emerge. Colloid diameter: $4.8\,\mu$m. Obstacle diameter: $10\,\mu$m. Field amplitude $E_0 = 2\,\text{V}/\mu\text{m}$.

4. Supplementary video 4: Evolution of the local roller current $|\mathbf{J}(x, y, t)|$ as a flock crosses the field of view. The rollers are focalized along a self-organized network of sparse flowing routes. Dark red color: no current, light red color: maximal current value. $\phi_\text{o} = 2 \times 10^{-2}$. Obstacle diameter: $10\,\mu$m. Field amplitude $E_0 = 2\,\text{V}/\mu\text{m}$. The current is defined as in Fig. 3a.

5. Supplementary video 5: A colloidal-roller flock cruises coherently through a square lattice of circular obstacles placed in a 15mm $\times$ 1mm rectangular chamber. Obstacle fraction: $\phi_\text{o} = 3 \times 10^{-2}$. Roller fraction: $\rho = 1.0 \times 10^{-2}$. Colloid diameter: $4.8\,\mu$m. Obstacle diameter: $10\,\mu$m. Field amplitude $E_0 = 2\,\text{V}/\mu\text{m}$.

# Supplementary References


[34] Bricard A., Caussin J.-B., Desreumaux N., Dauchot O. & Bartolo D. Emergence of macroscopic directed motion in populations of motile colloids. *Nature* **503**, 95–98 (2013).

[35] Bricard, A., Caussin, J.-B., Das, D., Savoie, C., Chikkadi, V., Shitara, K., Chepizhko, O., Peruani, F., Saintillan, D., & Bartolo, D. Emergent vortices in populations of colloidal rollers. *Nature Communications* **6**, 7470 (2015).

[36] Caussin, J.-B. & Bartolo, D. Tailoring the interaction between self-propelled bodies *Europhys. J. E* **37**, 55 (2014).

[37] Marchetti, M. C., Joanny, J. F., Ramaswamy, S., Liverpool, T. B., Prost, J., Rao, M. & Aditi Simha, R. Hydrodynamics of soft active matter. *Rev. Mod. Phys.* **85**, 1143–1189 (2013).

[38] Chepizhko, O. & Peruani, F. Diffusion, Subdiffusion, and Trapping of Active Particles in Heterogeneous Media. *Phys. Rev. Lett.* **111** 160604 (2013).

[39] Vicsek, T., Czirók, A., Ben-Jacob, E., Cohen, I. & Shochet, O. Novel Type of Phase Transition in a System of Self-Driven Particles. *Phys. Rev. Lett.*, **75**, 1226–1229 (1995).

[40] Grégoire, G. & Chaté, H. Onset of Collective and Cohesive Motion. *Phys. Rev. Lett.* **92** 025702 (2013).

[41] Solon, A., Chaté, H. & Tailleur, J. From Phase to Microphase Separation in Flocking Models: The Essential Role of Nonequilibrium Fluctuations, *Phys. Rev. Lett.* **114** 068101(2015).

[42] Peshkov, A., Bertin, E., Ginelli, F. & Chaté, H. Boltzmann-Ginzburg-Landau approach for continuous descriptions of generic Vicsek-like models. *Eur. Phys. J Special Topics* **223**, 1315 (2014).

[43] Toner, J. & Tu, Y. Long-Range Order in a Two-Dimensional Dynamical XY Model: How Birds Fly Together, *Phys. Rev. Lett.* **75** 4326–4329 (1995).

[44] Caussin, J.-B., Solon, A., Peshkov, A., Chaté, Dauxois, T., Tailleur, J., Vitelli, V. & Bartolo, D. Emergent spatial structures in flocking models: a dynamical system insight, *Phys. Rev. Lett.* **112** 148102 (2014).

[45] Solon, A., Caussin, J.-B., Bartolo, D., Chaté & Tailleur, J. Pattern formation in flocking models: A hydrodynamic description, *Phys. Rev. E* **92**, 062111 (2015).

[46] Bertin, E., Droz, M., & Grégoire, G. Hydrodynamic equations for self-propelled particles: microscopic derivation and stability analysis, *J. Phys. A: Math. Theor.* **42** 445001 (2009).

[47] Toner, J & Tu, Y. *To be published* (2016).
